# Supplementary material for: Reinforcement learning with Demonstrations from Mismatched Task under Sparse Reward
Source: arXiv:2212.01509 source file (2023-03-08)
Supplement: Supplementary file 1 [file 4appendix.tex]

\section{Appendix}
\subsection{Algorithm}

\begin{algorithm}
\begin{algorithmic}
\caption{CRSfD}
\STATE {\bfseries Input:} $Env$ Environment for the new task $M_i$; $\theta^{\pi}$ initial policy parameters; $\theta^{Q}$ initial action-value function parameters; $\theta^{Q'}$ initial target action-value function parameters; N target network update frequency.
\STATE {\bfseries Input:} $B^{E}$ replay buffer initialized with demonstrations. $B$ replay buffer initialized empty. $K$ number of pre-training gradient updates. $d$ expert buffer sample ratio. $batch$ mini batch size.
\STATE {\bfseries Input:} $\theta^{V}$ initial value function (potential function), original task discount factor $\gamma_0$.
\STATE {\bfseries Output:} $Q_{\theta}(s,a)$ action-value function (critic) and $\pi(.|s)$ the policy (actor).
\STATE \textcolor[rgb]{0,0.7,0}{\# Estimate value function from demonstration.}
\FOR{step $t$ {\bfseries in} \{0,1,2,...T\}}
\STATE Sample with $batch$ transitions from $B^{E}$, calculate their Monte-Carlo return with discount factor $\gamma_0$.
\STATE Estimate $V_{\theta}(s)$ conservatively by equation \ref{v_equation}
\ENDFOR
\STATE \textcolor[rgb]{0,0.7,0}{\# Interact with $Env$.}
\FOR{episode $e$ {\bfseries in} \{0,1,2,...M\}}

    \STATE Initialize state $s_0 \sim Env$
    \FOR{step $t$ {\bfseries in} episode length \{0,1,2,...T\}}
    \STATE Sample action from $\pi(.|s_t)$ 
    \STATE Get next state and natural sparse reward $s_{t+1},r_{t}$ 
    \STATE Shape reward by: $r_{t}'=r_{t}+\gamma_i V(s_{t+1},\theta^{V})-V(s_{t},\theta^{V})$ 
    \STATE Add single step transition $(s_t,a_t,r_t',s_{t+1})$ to replay buffer $B$.
    \ENDFOR

    \FOR{update step $l$ {\bfseries in} \{0,1,2,...L\}}
    \STATE Sample with prioritization: $d*batch$ transitions from $B^{E}$, $(1-d)*batch$ transitions from $B$. Concatenate them into a single batch. 
    \STATE Perform SAC update for actor and critic:$L_{Actor}(\theta^{\pi}), L_{Critic}(\theta^{Q})$.
    \IF{step $l \equiv 0 \pmod{N}$}
    \STATE Update target critic using moving average:$\theta^{Q'}=(1-\tau) \theta^{Q'}+\tau \theta^{Q}$
    \STATE Decrease expert buffer sample ratio: $d=d-\delta$ if $d>0$. 
    \ENDIF
    \ENDFOR

\ENDFOR
\end{algorithmic}
\end{algorithm}

\subsection{Implementation Details}
We implemented our CRSfD algorithm and the baseline algorithms in PyTorch and the implementation can be found in the supplementary materials. Simulated environments are based on robosuite framework \url{https://github.com/ARISE-Initiative/robosuite}. Our CRSfD algorithm is based on \url{https://github.com/denisyarats/pytorch_sac_ae} while baseline algorithms are based on \url{https://github.com/ikostrikov/pytorch-a2c-ppo-acktr-gail} and \url{https://github.com/ku2482/gail-airl-ppo.pytorch}.

\subsection{Videos}
Videos for simulated environments and real world environments can be found in the supplementary materials.

\subsection{Ablations}
As mentioned in section \ref{ablation}, we make two improvements over the reward shaping method to encourage the agent to explore around the demonstrations conservatively. (1) Regress value function of OOD states to zero. (2) Use a larger discount factor in new tasks. 

We ablate these 2 improvements and compare their performance on more environments, as show in Figure \ref{ablation_all}.

\begin{figure*}[ht]
\vspace{-3mm}
\begin{center}
\includegraphics[width=0.6\linewidth]{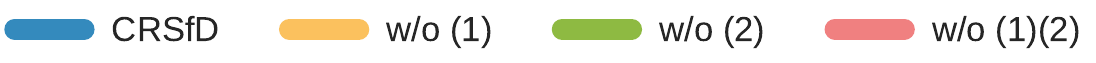}\\
\subfigure[Hole "1"]{
\includegraphics[width=0.23\linewidth]{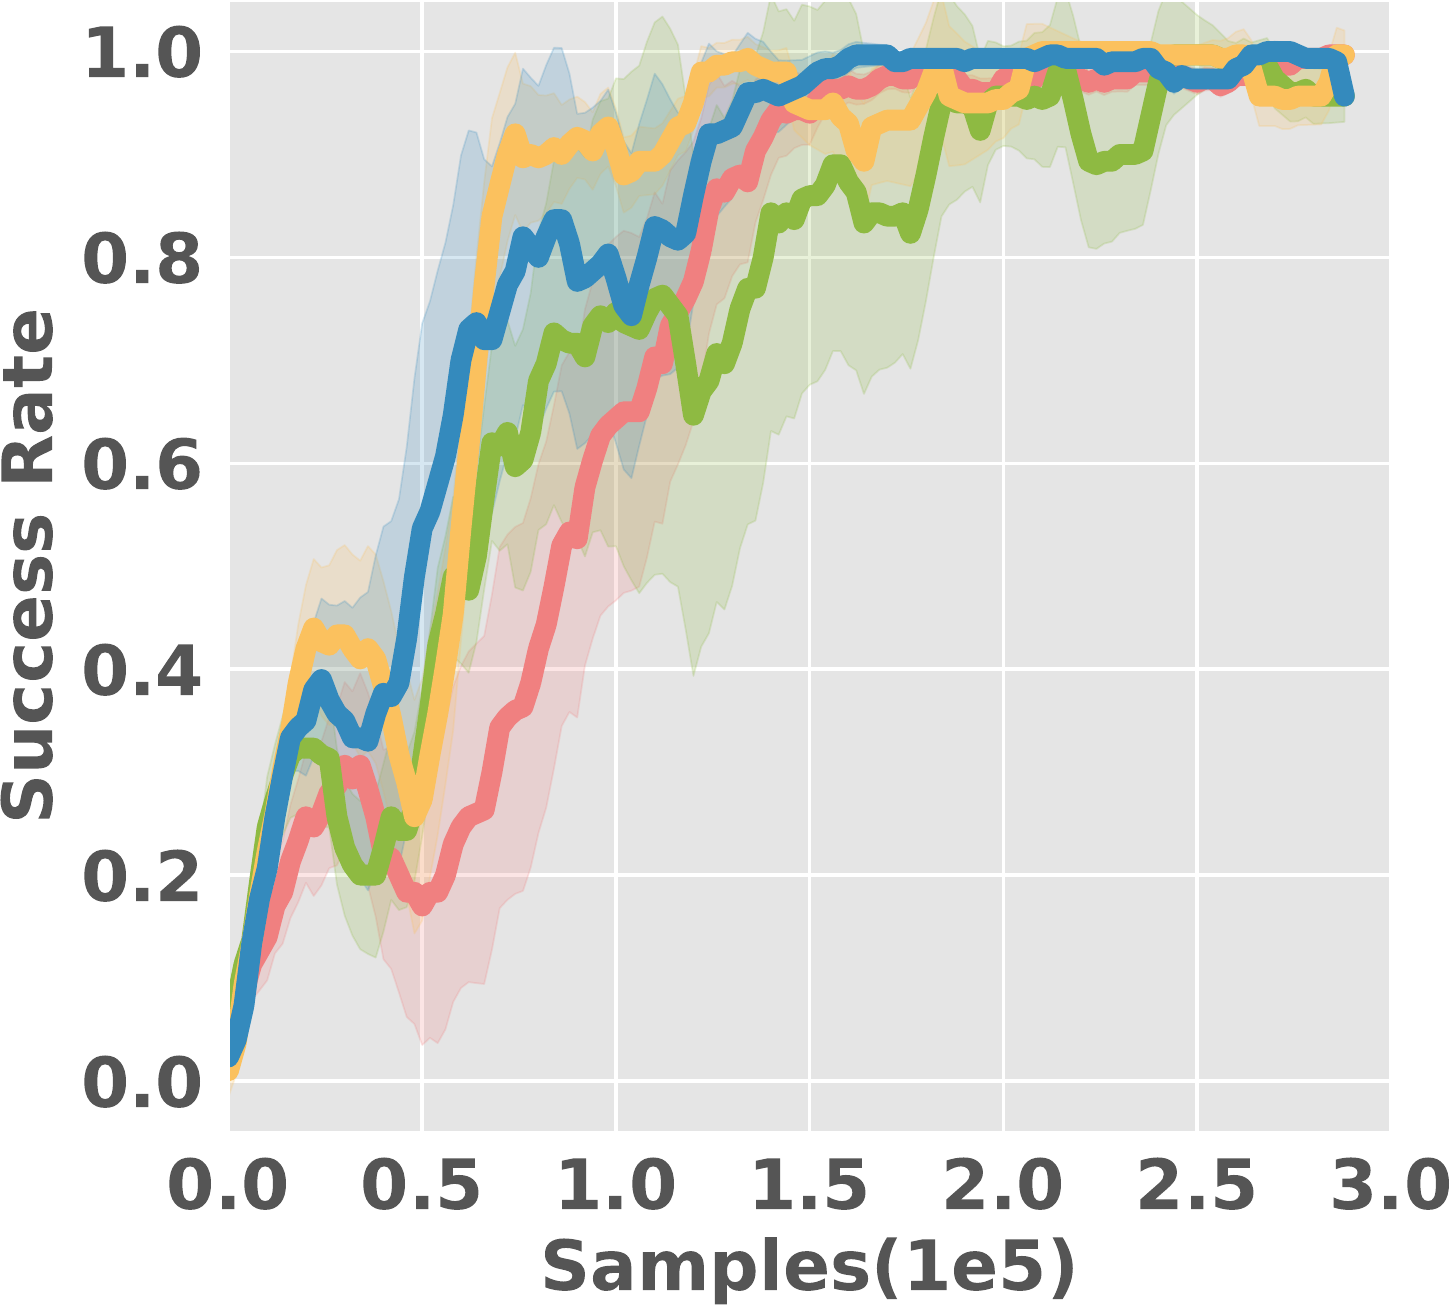}\vspace{0pt}}
\subfigure[Hole "2"]{
\includegraphics[width=0.23\linewidth]{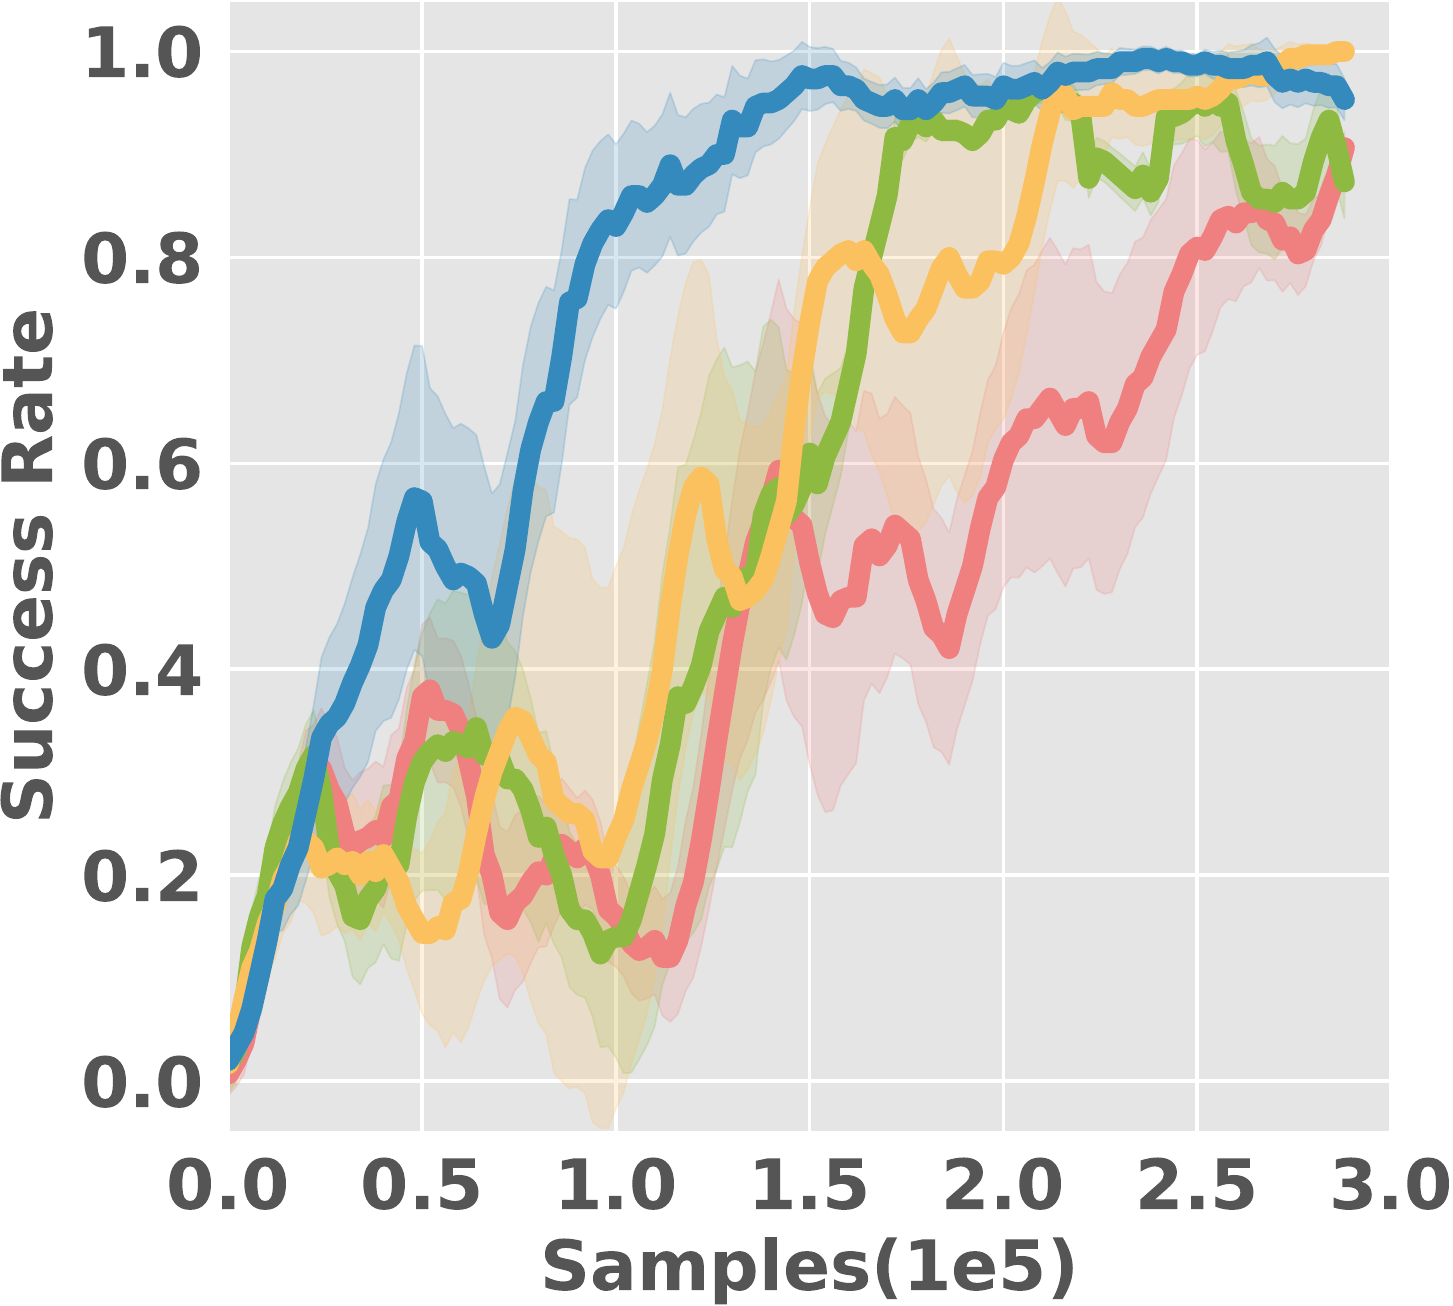}\vspace{0pt}}
\subfigure[Hole "3"]{
\includegraphics[width=0.23\linewidth]{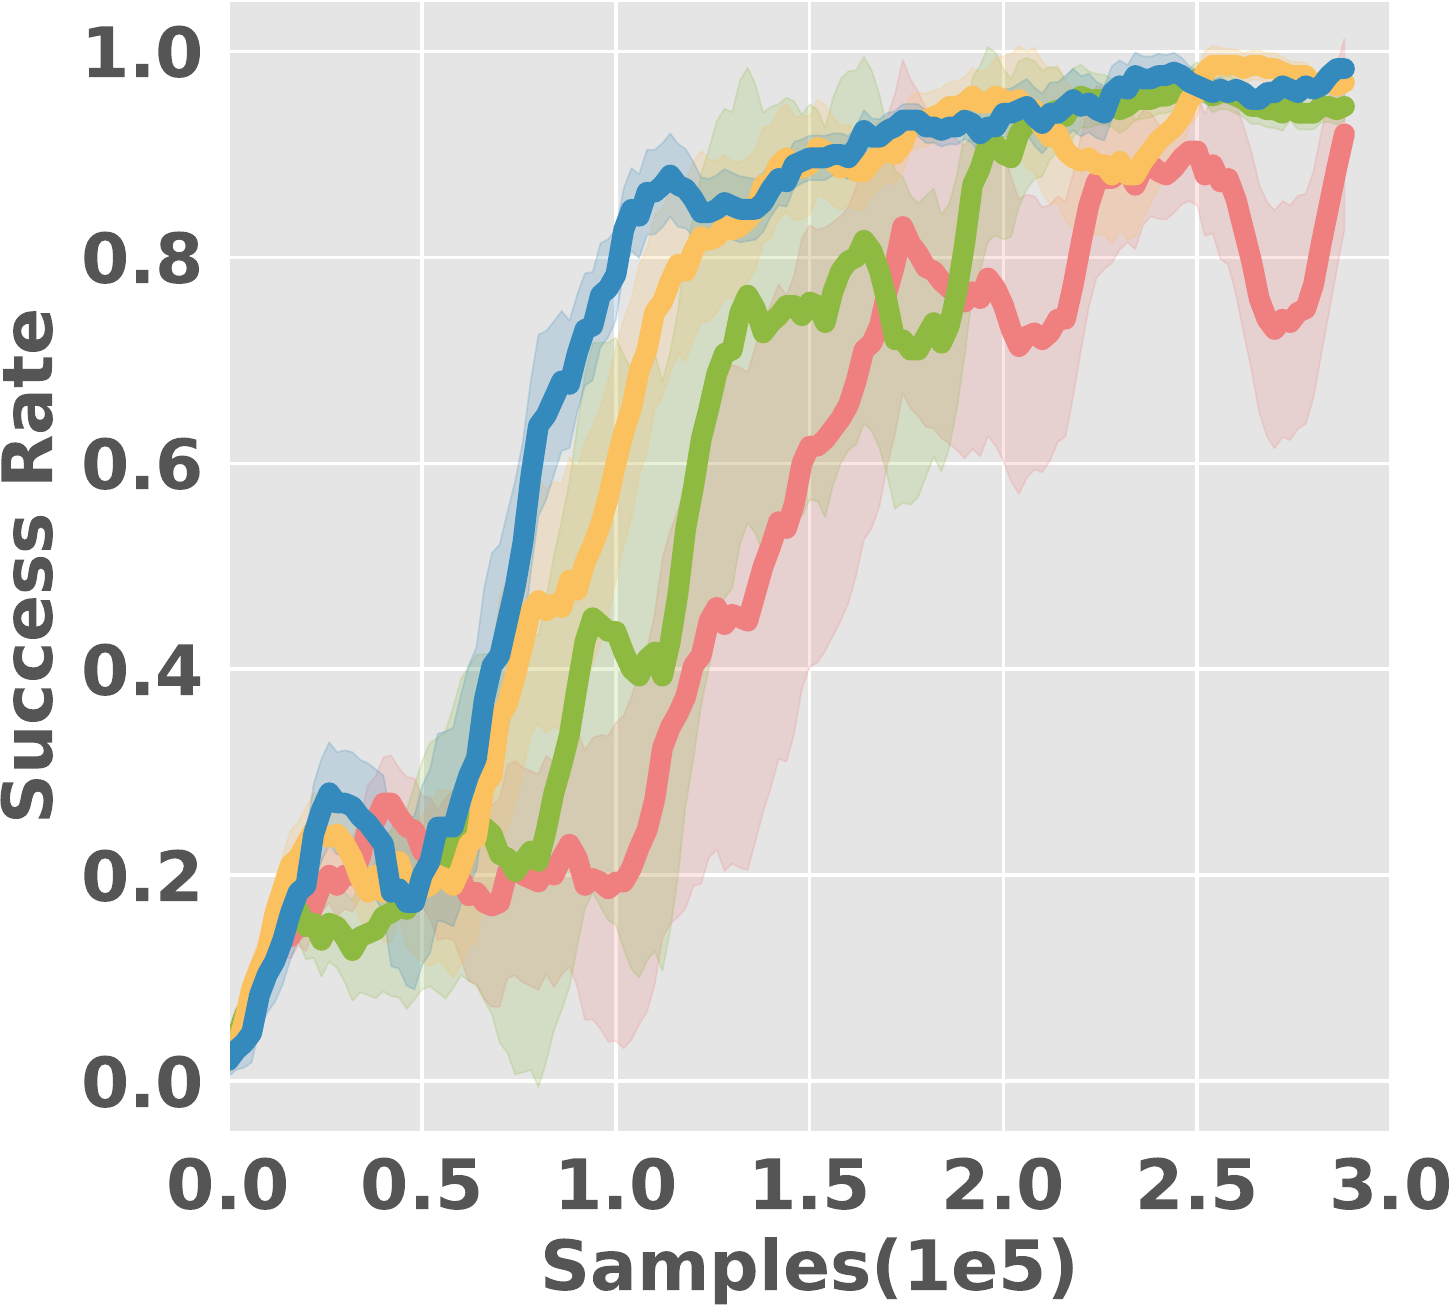}\vspace{0pt}}
\subfigure[Hole "4"]{
\includegraphics[width=0.23\linewidth]{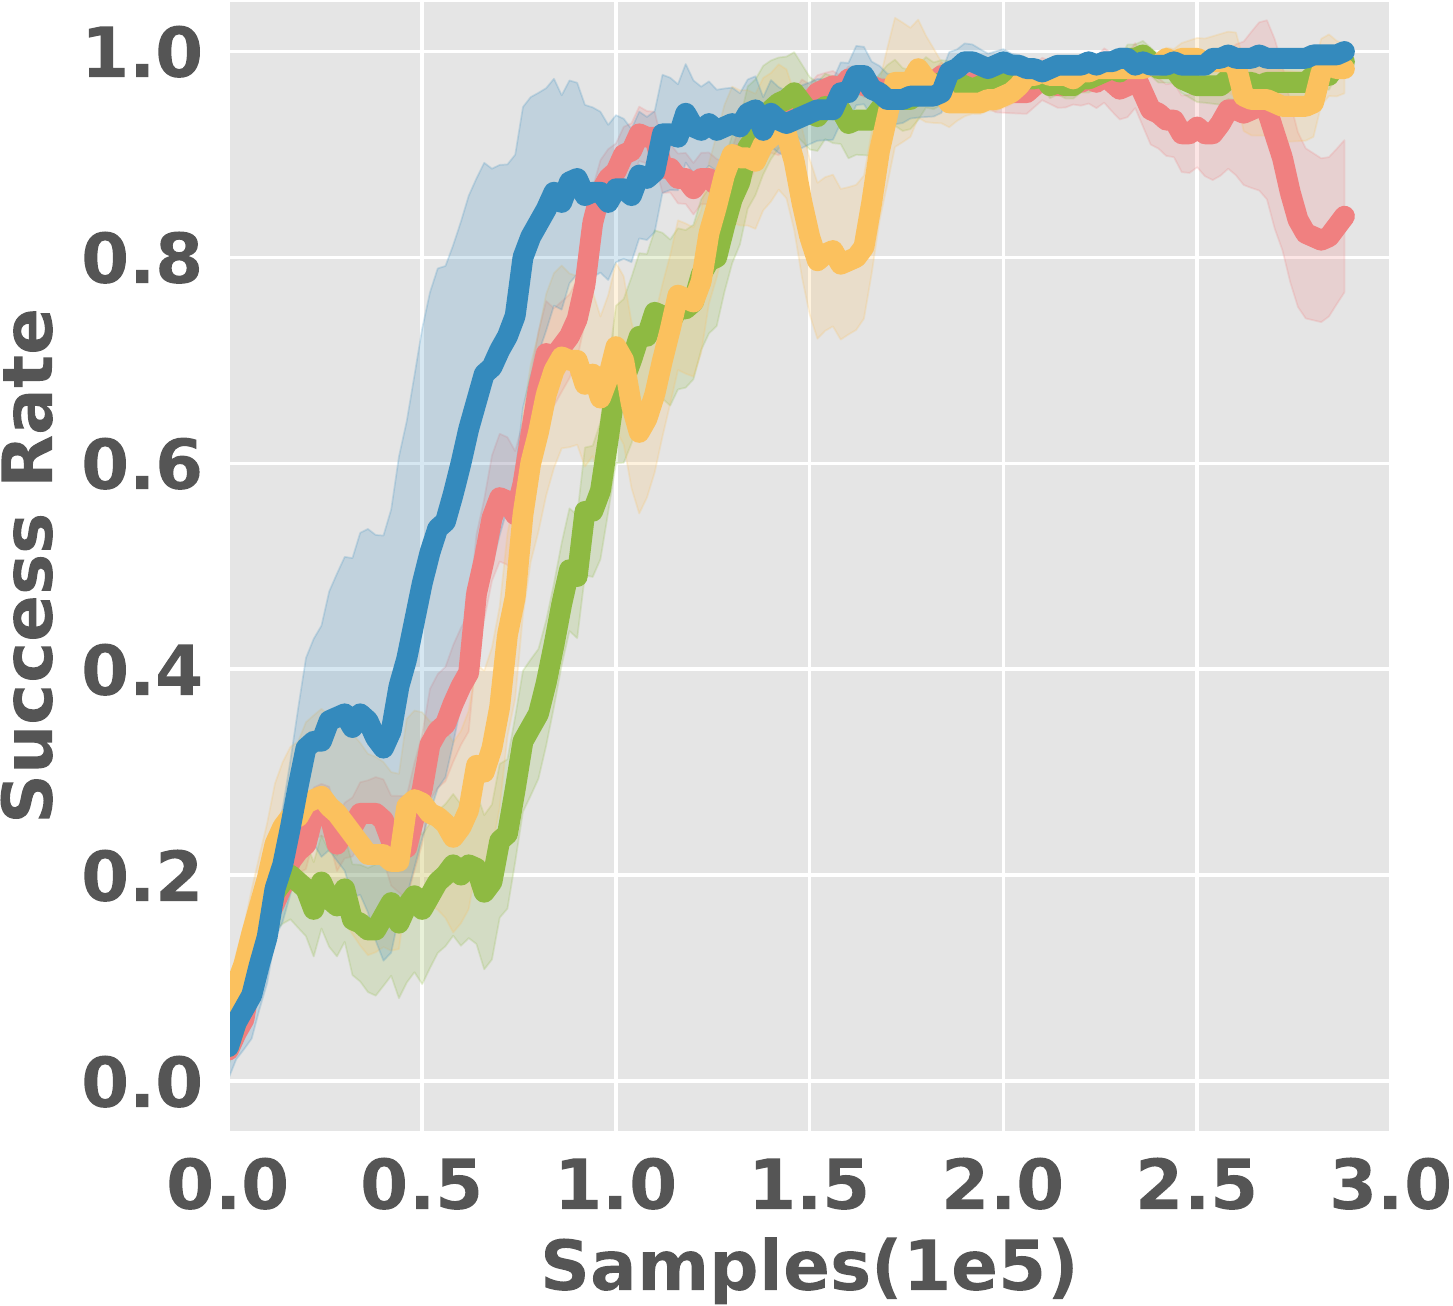}\vspace{0pt}}
\caption{Ablation studies of the conservativeness techniques. (1) means regressing value function to zero for OOD states. (2) means setting larger discount factors. }
\label{ablation_all}
\end{center}
\vspace{-5mm}
\end{figure*}

\setcounter{theorem}{0}
\subsection{Proof for theorem}
\begin{theorem}
For task $M_0$ with transition $T_0$ and new task $M_k$ with transition $T_k$, define total variation divergence $D_{TV}(s,a)=\Sigma_{s'}|T_0(s'|s,a)-T_k(s'|s,a)|=\delta$. If we have  $\delta<(\gamma_k-\gamma_0) \mathbb{E}_{T_2(s'|s,a)}[ V_{M_0}^D(s')]/\gamma_0 \max_{s'}V_{M_0}^D(s')$, then 
following the expert policy in new task will result in immediate reward greater then 0:
\begin{equation}
\setlength{\abovedisplayskip}{0pt}
\setlength{\belowdisplayskip}{0pt}
    \mathbb{E}_{a\sim \pi(.|s)}r'(s,a)
    \geq (\gamma_k-\gamma_0)\mathbb{E}_{T_{k}(s'|s)}[ V_{M_0}^{D}(s')]-\gamma_0 \delta \max_{s'}V_{M_0}^D(s') > 0
\end{equation}
\end{theorem}

\textbf{Proof:}
For simplify, denote demonstration state value function in original task $V_{M_0}^D=V_1(s)$.
Start from the reward shaping equations, and extend $V_1(s)$ for one more time step:
\begin{equation}
\begin{split}
    r'(s,a,s')=&r(s,a,s')+\gamma_k V_1(s’)- V_1(s)\\
    r'(s,a)=&r(s,a)+\gamma_k \mathbb{E}_{T_k(s'|s,a)}[ V_1(s')]-V_1(s)\\
    =&(\gamma_k-\gamma_0)\mathbb{E}_{T_k(s'|s,a)}[ V_1(s')]+ \left(r(s,a)+\gamma_0 \mathbb{E}_{T_k(s'|s,a)}[ V_1(s')]-V_1(s) \right)\\
    \geq&(\gamma_k-\gamma_0)\mathbb{E}_{T_k(s'|s,a)}[ V_1(s')]+\left(Q^{\pi_1}(s,a)-V_1(s)\right)- \gamma_0 \delta \max_{s'}V_1(s')
\end{split}
\end{equation}
Take expectation on demonstration policies:
\begin{equation}
\begin{split}
    \mathbb{E}_{a\sim \pi(.|s)}r'(s,a)
    \geq& \mathbb{E}_{a\sim \pi(.|s)}\left[(\gamma_k-\gamma_0)\mathbb{E}_{T_k(s'|s,a)}[ V_1(s')]\right]- \gamma_0 \delta \max_{s'}V_1(s')
\end{split}
\end{equation}
For a sparse reward environment, we have $r(s,a)=0$ almost everywhere:
\begin{equation}
\begin{split}
    \mathbb{E}_{a\sim \pi(.|s)}r'(s,a)
    \geq &\mathbb{E}_{a\sim \pi(.|s)}\left[(\gamma_k-\gamma_0)\mathbb{E}_{T_k(s'|s,a)}[ V_1(s')]\right]- \gamma_0 \delta \max_{s'}V_1(s')\\
    =&(\gamma_k-\gamma_0)\mathbb{E}_{T_{k}(s'|s)}[ V_1(s')]-\gamma_0 \delta \max_{s'}V_1(s')
\end{split}
\end{equation}

\subsection{Increasingly Larger Task Mismatch}

\begin{figure}[H]
% \vspace{-4mm}
\begin{center}
\includegraphics[width=1.0\linewidth]{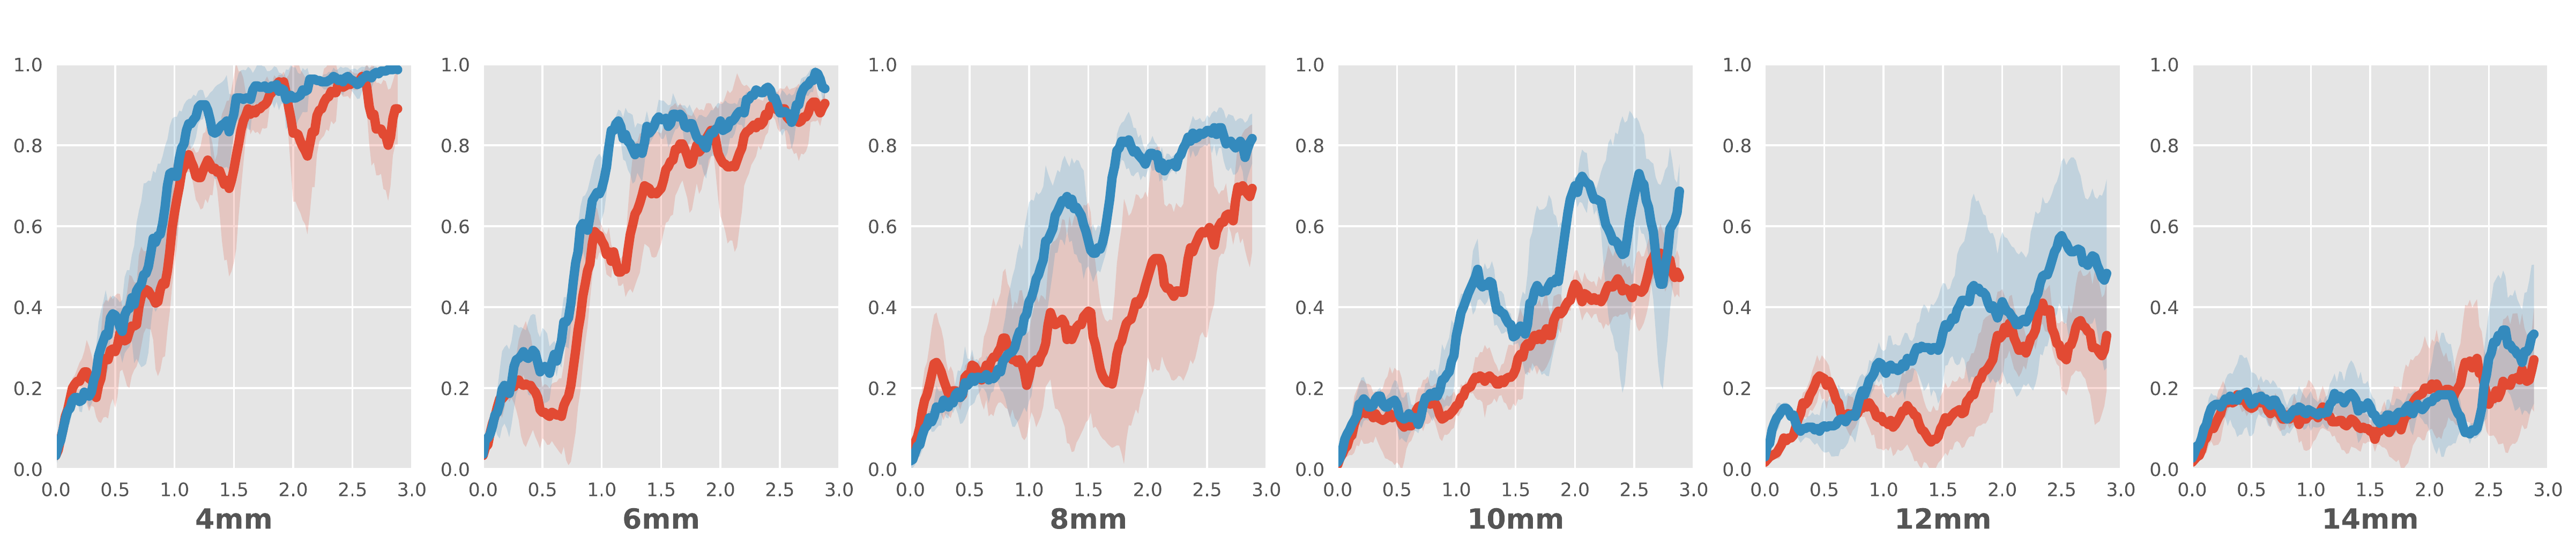}
\caption{Increasingly larger task mismatch. Experiments are done on hole shape 0 with increasing random hole position.}
\label{setting3}
\end{center}
\vspace{-5mm}
\end{figure}

We can observe that as task difference increases, our method first gradually outperforms baseline methods. When task mismatch are too large, our method gradually loss some performance and has similar performance with baselines.
